# Supplementary material for: Metals, fractional metals, and superconductivity in rhombohedral trilayer graphene
Source: arXiv:2109.04466 ancillary file (2022-02-15)
Supplement: Supplementary file 1 [file RTLG_Supplementary.pdf]

# Supplementary Material: Parent (half)metal and emergent superconductivity in rhombohedral trilayer graphene

András L. Szabó[1] and Bitan Roy[2]

[1]*Max-Planck-Institut für Physik komplexer Systeme, Nöthnitzer Str. 38, 01187 Dresden, Germany*
[2]*Department of Physics, Lehigh University, Bethlehem, Pennsylvania, 18015, USA*

(Dated: January 9, 2022)

The Supplementary Material contains: (1) Definition of Nambu-doubled spinor. (2) Calculation of triplet pairing susceptibilities in a half-metal, relevant to SC2. (3) Calculation of susceptibilities of the isospin coherent paramagnetic order parameters, relevant to SC1. (4) Details of the renormalization group (RG) analysis as it pertains to the competition of valence bond order (VBO) and $s$-wave pairing in the vicinity of SC1. (5) RG analysis showing emergence of $f$-wave pairing from antiferromagnet interaction with the assistance of external electric field. (6) Quantum anomalous Hall order and resulting quarter-metal.

## S1. NAMBU-DOUBLED SPINOR

The sixteen-component Nambu doubled spinor in rhombohedral trilayer graphene is defined as

$$\Psi_{\text{Nam}} = \begin{pmatrix} \Psi_{\omega,\boldsymbol{k}} \\ \Gamma_{210}\Psi^{*}_{-\omega,-\boldsymbol{k}} \end{pmatrix}, \tag{S1}$$

where in the lower block we absorbed the unitary part of the time reversal operator $U = \Gamma_{210} \equiv \sigma_2\tau_1\beta_0$. The eight-component spinor is

$$\Psi_{\omega,\boldsymbol{k}} = \left[c_{\uparrow}^{+K}, c_{\uparrow}^{-K}, c_{\downarrow}^{+K}, c_{\downarrow}^{-K}\right]^{\top}, \text{ with } c_s^v = \left[a_{3,s}^v, b_{1,s}^v\right](\omega). \tag{S2}$$

Here $r^v_{j,s}(\omega)$ are annihilation operators for fermions on the $a_3$ and $b_1$ sublattices with valley index $v = \pm\boldsymbol{K}$, Matsubara frequency $\omega$ and spin projection $s =\uparrow,\downarrow$, and $\top$ denotes transposition. In the main manuscript $\Psi \equiv \Psi_{\text{Nam}}$.

## S2. MEAN FIELD SUSCEPTIBILITY OF TRIPLET PAIRING ORDERS

In this section we present the computation of the mean field susceptibility of candidate triplet pairing orders for SC2. These are the $f$-wave pairing ($A_{1u}$), pair-density-wave ($A_{2\mathbf{K}}$), spin nematic ($E_u$) and a gapless pairing ($A_{2g}$). The corresponding irreducible representation of the $D_{3d}$ group is shown in parentheses. The bare mean field susceptibility for zero external frequency and momentum is shown in Eq. (3) of the main text. Performing the matrix algebra we obtain for the susceptibilities of the candidate triplet pairings

$$\chi_{A_{1u}} = 8(-\tilde{I}_\omega + \tilde{I}_u + 2\tilde{I}_f), \quad \chi_{A_{2\mathbf{K}}} = 8(-\tilde{I}_\omega - \tilde{I}_u + 2\tilde{I}_f), \quad \chi_{E_u} = 8(-\tilde{I}_\omega - \tilde{I}_u), \quad \chi_{A_{2g}} = 8(-\tilde{I}_\omega + \tilde{I}_u - 2\tilde{I}_f), \tag{S3}$$

where we wrote the contributions on the right-hand side in terms of integrals $\tilde{I}_x \equiv \tilde{I}_x(u_{\text{eff}}, t, \mu)$ for $x = \omega, u, f$, the explicit forms of which are

$$\begin{aligned}
\tilde{I}_\omega(u_{\text{eff}}, t, \mu) &= \frac{1}{(2\pi)^2}\int_0^\infty \mathrm{d}k\, k \int \mathrm{d}\phi_k T \sum_{\omega_n} \frac{(i\omega_n - \mu)(i\omega_n + \mu)}{[(i\omega_n - \mu)^2 - \epsilon_{\boldsymbol{k}}^2][(i\omega_n + \mu)^2 - \epsilon_{\boldsymbol{k}}^2]} = \frac{1}{8\pi\alpha\Lambda}\int_0^\infty \mathrm{d}k\, k\, \tilde{F}_\omega(k, u_{\text{eff}}, t, \mu), \\
\tilde{I}_u(u_{\text{eff}}, t, \mu) &= \frac{1}{(2\pi)^2}\int_0^\infty \mathrm{d}k\, k \int \mathrm{d}\phi_k T \sum_{\omega_n} \frac{u^2}{[(i\omega_n - \mu)^2 - \epsilon_{\boldsymbol{k}}^2][(i\omega_n + \mu)^2 - \epsilon_{\boldsymbol{k}}^2]} = \frac{1}{8\pi\alpha\Lambda} u^2 \int_0^\infty \mathrm{d}k\, k\, \tilde{F}(k, u_{\text{eff}}, t, \mu), \\
\tilde{I}_f(u_{\text{eff}}, t, \mu) &= \frac{1}{(2\pi)^2}\int_0^\infty \mathrm{d}k\, k \int \mathrm{d}\phi_k T \sum_{\omega_n} \frac{f_i^2(\boldsymbol{k})}{[(i\omega_n - \mu)^2 - \epsilon_{\boldsymbol{k}}^2][(i\omega_n + \mu)^2 - \epsilon_{\boldsymbol{k}}^2]} = \frac{1}{8\pi\alpha\Lambda}\frac{1}{2}\int_0^\infty \mathrm{d}k\, k^7 \tilde{F}(k, u_{\text{eff}}, t, \mu).
\end{aligned} \tag{S4}$$

Here $\epsilon_{\boldsymbol{k}} = \sqrt{\alpha^2 k^6 + u_{\text{eff}}^2}$, $f_1(\boldsymbol{k}) = k^3\cos(3\phi_k)$, $f_2(\boldsymbol{k}) = k^3\sin(3\phi_k)$, with $\phi_k = \arctan(k_y/k_x)$. We have also rescaled $k/\Lambda \to k$, where $\Lambda$ bears the dimension of momentum. Therefore, the two $f$-wave harmonics yield identical contributions after the angular integration. The fermionic Matsubara frequencies are $\omega_n = (2n+1)\pi T$ with $n$ as an integer.

The alternating sign of $\mu$ is due to the off-diagonal structure of the pairing matrices in the particle-hole subspace. The functions appearing on the right-hand-side of Eq. (S4) read

$$\tilde{F}_\omega(k,u_{\rm eff},t,\mu)=\sum_{\tau=\pm}\frac{\tanh\left(\frac{\sqrt{k^6+u_{\rm eff}^2}+\tau\mu}{2t}\right)\left[-\tau(k^6+u_{\rm eff}^2)-\sqrt{k^6+u_{\rm eff}^2}\mu+\tau 2\mu^2\right]}{2\mu(k^6+u_{\rm eff}^2-\mu^2)},$$
$$\tilde{F}(k,u_{\rm eff},t,\mu)=\sum_{\tau=\pm}\frac{\tanh\left(\frac{\sqrt{k^6+u_{\rm eff}^2}+\tau\mu}{2t}\right)\left[-\tau\sqrt{k^6+u_{\rm eff}^2}+\mu\right]}{2\mu\sqrt{k^6+u_{\rm eff}^2}(k^6+u_{\rm eff}^2-\mu^2)}. \tag{S5}$$

We here measure $T$, $\mu$, and $u_{\rm eff}$ in units of $\alpha$ and $\Lambda$, and redefine these quantities according to

$$T/(\alpha\Lambda^3)\to t,\qquad \mu/(\alpha\Lambda^3)\to\mu,\qquad u_{\rm eff}/(\alpha\Lambda^3)\to u_{\rm eff}. \tag{S6}$$

The parameters $t$, $\mu$ and $u_{\rm eff}$ are now dimensionless. Note, due to the cubic dispersion the above integrals are in fact ultraviolet convergent, whereas the infrared divergence is avoided due to finite temperature and the presence of finite $u_{\rm eff}$. The triplet pairing susceptibilities are plotted against $u_{\rm eff}$ for fixed $t$ and $\mu$ in Fig. 3(a) of the main text.

## S3. MEAN FIELD SUSCEPTIBILITY OF EXCITONIC ORDERS

Next we move on to assess the susceptibilities of excitonic parent state candidates for the pairing phase SC1. These describe an isospin coherent paramagnetic metal, leaving three options, the valence bond order (VBO), bond current (BC) and smectic charge-density-wave (sCDW). The corresponding order parameters transform under the $A_{1\mathbf{K}}$, $A_{2\mathbf{K}}$, and $E_{\mathbf{K}}$ representations of the $D_{3d}$ group, respectively. The susceptibilities read

$$\chi_{\rm VBO}=8(-I_\omega+I_u+2I_f),\qquad \chi_{\rm BC}=8(-I_\omega+I_u-2I_f),\qquad \chi_{\rm sCDW}=8(-I_\omega-I_u), \tag{S7}$$

where we once again write the contributions in terms of integrals over $|\boldsymbol{k}|$. These are of the explicit form

$$I_\omega(u,t,\mu)=\frac{1}{(2\pi)^2}\int_0^\infty {\rm d}k\,k\int {\rm d}\phi_k T\sum_{\omega_n}\frac{(i\omega_n-\mu)^2}{[(i\omega_n-\mu)^2-\epsilon_{\boldsymbol{k}}^2]^2}=\frac{1}{8\pi\alpha\Lambda}\int_0^\infty {\rm d}k\,k\,F_\omega(k,u,t,\mu),$$
$$I_u(u,t,\mu)=\frac{1}{(2\pi)^2}\int_0^\infty {\rm d}k\,k\int {\rm d}\phi_k T\sum_{\omega_n}\frac{u^2}{[(i\omega_n-\mu)^2-\epsilon_{\boldsymbol{k}}^2]^2}=\frac{1}{8\pi\alpha\Lambda}u^2\int_0^\infty {\rm d}k\,k\,F(k,u,t,\mu),$$
$$I_f(u,t,\mu)=\frac{1}{(2\pi)^2}\int_0^\infty {\rm d}k\,k\int {\rm d}\phi_k T\sum_{\omega_n}\frac{f_i^2(\boldsymbol{k})}{[(i\omega_n-\mu)^2-\epsilon_{\boldsymbol{k}}^2]^2}=\frac{1}{8\pi\alpha\Lambda}\frac{1}{2}\int_0^\infty {\rm d}k\,k^7F(k,u,t,\mu). \tag{S8}$$

where the appearing functions read

$$F_\omega(k,u,t,\mu)=-\sum_{\tau=\pm}\left[\frac{{\rm sech}^2\left(\frac{\sqrt{k^6+u^2}+\tau\mu}{2t}\right)}{4t}+\frac{\tanh\left(\frac{\sqrt{k^6+u^2}+\tau\mu}{2t}\right)}{2\sqrt{k^6+u^2}}\right],$$
$$F(k,u,t,\mu)=-\sum_{\tau=\pm}\left[\frac{{\rm sech}^2\left(\frac{\sqrt{k^6+u^2}+\tau\mu}{2t}\right)}{4t(k^6+u^2)}-\frac{\tanh\left(\frac{\sqrt{k^6+u^2}+\tau\mu}{2t}\right)}{2(k^6+u^2)^{\frac{3}{2}}}\right]. \tag{S9}$$

Here we again used rescaled quantities defined in Eq. (S6), as well as $u/(\alpha\Lambda^3)\to u$. The susceptibilities are plotted against $u$ for fixed $t$ and $\mu$ in Fig. 4(a) of the main text.

## S4. RENORMALIZATION GROUP (RG) ANALYSIS: FROM VBO TO $s$-WAVE PAIRING

Here we present in details the RG flow equations in the context of competing VBO ($A_{1\mathbf{K}}$) and $s$-wave pairing ($A_{1g}$) as it pertains to SC1. In Eq. (4) of the main text we summarized the $\beta$-functions of the dimensionless interaction coupling $\lambda_{A_{1\mathbf{K}}}$, as well as those of dimensionless temperature, chemical potential and interlayer voltage bias. They respectively read

$$\frac{{\rm d}\lambda_{A_{1\mathbf{K}}}}{{\rm d}\ell}=\lambda_{A_{1\mathbf{K}}}+16(I_u^\Lambda+2I_f^\Lambda)\lambda_{A_{1\mathbf{K}}}^2,\qquad \frac{{\rm d}t}{{\rm d}\ell}=3t,\qquad \frac{{\rm d}\mu}{{\rm d}\ell}=3\mu,\qquad \frac{{\rm d}u}{{\rm d}\ell}=3u. \tag{S10}$$

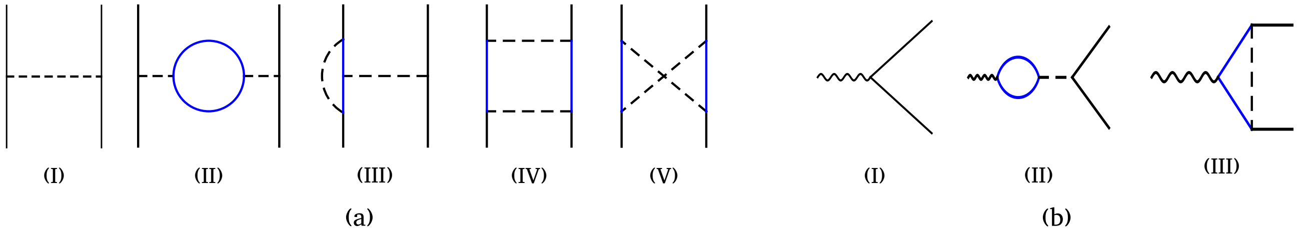


Figure S1. (a) Feynman diagrams yielding renormalization of quartic coupling. (aI) Bare four-fermion interaction vertex. Feynman diagrams (aII)-(aV) yield corrections to the bare interaction vertex to the leading order. Here, solid lines represent fermions. While the blue lines in (aII)-(aV) correspond to the fast modes, living within a thin Wilsonian momentum shell $\Lambda\, e^{-\ell} < |\mathbf{k}| < \Lambda$, where $\Lambda$ is the ultraviolet momentum cut-off and $\ell$ is the logarithm of the renormalization group scale, the black solid lines are the slow modes with $|\mathbf{k}| < \Lambda\, e^{-\ell}$. (b) Feynman diagrams yielding renormalization of conjugate field. (bI) The bare vertex associated with the source term $\Psi^\dagger O \Psi$. The leading order renormalization of such vertex arises from Feynman diagrams (bII) and (bIII), yielding the RG flow of the source terms or conjugate fields. Here, wavy lines stand for the conjugate field, while solid lines for fermions, and the dashed lines for the interaction vertex.

On the other hand, the RG flow equations of the corresponding susceptibilities from Eq. (5) of the main text are of the explicit form

$$\frac{\mathrm{d}\ln\Delta_{A_1\mathbf{K}}}{\mathrm{d}\ell} - 3 = 16(I_u^\Lambda + 2I_f^\Lambda)\lambda_{A_1\mathbf{K}}, \qquad \frac{\mathrm{d}\ln\Delta_{A_{1g}}}{\mathrm{d}\ell} - 3 = 4(\tilde{I}_u^\Lambda + 2\tilde{I}_f^\Lambda - \tilde{I}_\omega^\Lambda)\lambda_{A_1\mathbf{K}}, \tag{S11}$$

where once again we wrote the contributions in terms of integrals. Note the RG is performed by integrating out only the momentum shell $\Lambda e^{-\ell} < |\boldsymbol{k}| < \Lambda$, where $\Lambda$ is a nonuniversal ultraviolet cutoff and $\ell$ is the logarithm of the RG scale. We indicate the shell integration with the superscript $\Lambda$, and in the $\beta$-functions we suppress the dependence of them on $t$, $\mu$, and $u$. The integrals are written as

$$\begin{aligned} I_\omega^\Lambda(u,t,\mu) &= \frac{1}{4}F_\omega^\Lambda(u,t,\mu), & I_u^\Lambda(u,t,\mu) &= \frac{1}{4}u^2F^\Lambda(u,t,\mu), & I_f^\Lambda(u,t,\mu) &= \frac{1}{4}\frac{1}{2}F^\Lambda(u,t,\mu), \\ \tilde{I}_\omega^\Lambda(u,t,\mu) &= \frac{1}{4}\tilde{F}_\omega^\Lambda(u,t,\mu), & \tilde{I}_u^\Lambda(u,t,\mu) &= \frac{1}{4}u^2\tilde{F}^\Lambda(u,t,\mu), & \tilde{I}_f^\Lambda(u,t,\mu) &= \frac{1}{4}\frac{1}{2}\tilde{F}^\Lambda(u,t,\mu). \end{aligned} \tag{S12}$$

Even though $I_\omega^\Lambda(u,t,\mu)$ does not appear in the above $\beta$-functions, we include it here for the sake of completeness. The appearing functions are of the form

$$\begin{aligned} F_\omega^\Lambda(u,t,\mu) &= -\sum_{\tau=\pm}\left[\frac{\mathrm{sech}^2\left(\frac{\sqrt{1+u^2}+\tau\mu}{2t}\right)}{4t} + \frac{\tanh\left(\frac{\sqrt{1+u^2}+\tau\mu}{2t}\right)}{2\sqrt{1+u^2}}\right], \\ F^\Lambda(u,t,\mu) &= -\sum_{\tau=\pm}\left[\frac{\mathrm{sech}^2\left(\frac{\sqrt{1+u^2}+\tau\mu}{2t}\right)}{4t(1+u^2)} - \frac{\tanh\left(\frac{\sqrt{1+u^2}+\tau\mu}{2t}\right)}{2(1+u^2)^{\frac{3}{2}}}\right], \\ \tilde{F}_\omega^\Lambda(u,t,\mu) &= \sum_{\tau=\pm}\frac{\tanh\left(\frac{\sqrt{1+u^2}+\tau\mu}{2t}\right)\left[-\tau(1+u^2) - \sqrt{1+u^2}\mu + \tau 2\mu^2\right]}{2\mu(1+u^2-\mu^2)}, \\ \tilde{F}^\Lambda(u,t,\mu) &= \sum_{\tau=\pm}\frac{\tanh\left(\frac{\sqrt{1+u^2}+\tau\mu}{2t}\right)\left[-\tau\sqrt{1+u^2} + \mu\right]}{2\sqrt{1+u^2}\mu(1+u^2-\mu^2)}, \end{aligned} \tag{S13}$$

where we introduced dimensionless variables according to

$$\frac{g_{A_1\mathbf{K}}}{2\pi\alpha\Lambda} \to \lambda_{A_1\mathbf{K}}, \qquad \frac{T}{\alpha\Lambda^3} \to t, \qquad \frac{\mu}{\alpha\Lambda^3} \to \mu, \qquad \frac{u}{\alpha\Lambda^3} \to u. \tag{S14}$$

## S5. RG ANALYSIS: FROM LAYER ANTIFERROMAGNET TO $f$-WAVE PAIRING

Next we consider the effects of layer polarization augmented with electronic interaction in the LAF channel, which is the dominant component of on-site Hubbard repulsion. We show that these combined effects are conducive for

the realization of spin-triplet $f$-wave pairing, emerging from the parent spin-polarized, valley-unpolarized half-metal. The band structure is described by the Hamiltonian Eq. (1) of the main text. Here, the cubic bands are gapped due to the external $u$ field, and depending on the magnitude of chemical potential $\mu$ we realize an insulator ($\mu < u$) or a metal ($\mu > u$). Interactions are described by the quartic term

$$g_{A_{2u}} \sum_{s=1}^{3} (\Psi^\dagger \Gamma_{0s03} \Psi)^2. \tag{S15}$$

Once again we introduce dimensionless coupling constant according to

$$\frac{g_{A_{2u}}}{32\pi\alpha\Lambda} \to \lambda_{A_{2u}}, \tag{S16}$$

and the corresponding RG flow equation reads

$$\frac{\mathrm{d}\lambda_{A_{2u}}}{\mathrm{d}\ell} = \lambda_{A_{2u}} + 4(10 I_f^\Lambda - 4 I_u^\Lambda - \tilde{I}_u^\Lambda)\lambda_{A_{2u}}^2. \tag{S17}$$

The candidate ordered phases in the presence of repulsive $\lambda_{A_{2u}}$ are LAF ($A_{2u}$), $E_g$ nematic pairing, and $f$-wave pairing ($A_{1u}$). The flow equations of the corresponding conjugate $\Delta$ fields are of the form

$$\frac{\mathrm{d}\ln\Delta_{A_{2u}}}{\mathrm{d}\ell} - 3 = 18(2I_f^\Lambda - I_u^\Lambda)\lambda_{A_{2u}}, \qquad \frac{\mathrm{d}\ln\Delta_{E_g}}{\mathrm{d}\ell} - 3 = -6(\tilde{I}_u^\Lambda + \tilde{I}_\omega^\Lambda)\lambda_{A_{2u}},$$
$$\frac{\mathrm{d}\ln\Delta_{A_{1u}}}{\mathrm{d}\ell} - 3 = 2(\tilde{I}_u^\Lambda + 2\tilde{I}_f^\Lambda - \tilde{I}_\omega^\Lambda)\lambda_{A_{2u}}. \tag{S18}$$

## S6. QUANTUM ANOMALOUS HALL ORDER AND QUARTER-METAL

The effective single-particle Hamiltonian in the presence of external displacement field induced layer polarization ($u$), Hubbard repulsion ($U$) driven layer antiferromagnet ($\Delta_{\rm LAF}$) and intralayer next-nearest-neighbor repulsion ($V_2$) driven quantum anomalous Hall order ($\Delta_{\rm QAH}$) reads

$$H_{\rm QM} = \alpha\left[f_1(\boldsymbol{k})\Gamma_{3031} + f_2(\boldsymbol{k})\Gamma_{3002}\right] + u\Gamma_{3003} + \Delta_{\rm LAF}\Gamma_{0303} + \Delta_{\rm QAH}\Gamma_{0033} - \mu\Gamma_{3000}. \tag{S19}$$

The energy spectra of this Hamiltonian are $\pm E_j - \mu$, where for $j = 1,2,3,4$ we find

$$E_1 = \sqrt{\alpha^2|\boldsymbol{k}|^2 + (u + \Delta_{\rm LAF} + \Delta_{\rm QAH})^2}, \quad E_2 = \sqrt{\alpha^2|\boldsymbol{k}|^2 + (u - \Delta_{\rm LAF} + \Delta_{\rm QAH})^2},$$
$$E_3 = \sqrt{\alpha^2|\boldsymbol{k}|^2 + (u + \Delta_{\rm LAF} - \Delta_{\rm QAH})^2}, \quad E_4 = \sqrt{\alpha^2|\boldsymbol{k}|^2 + (u - \Delta_{\rm LAF} - \Delta_{\rm QAH})^2}. \tag{S20}$$

Therefore, the spectra loose both valley and spin degeneracy. When the chemical potential ($\mu$) is such that

$$|u - \Delta_{\rm LAF} - \Delta_{\rm QAH}| < \mu < |u - \Delta_{\rm LAF} + \Delta_{\rm QAH}| \tag{S21}$$

the system supports a quarter-metal with only one type of carrier. Here we assumed $\Delta_{\rm LAF} > \Delta_{\rm QAH}$, as $\Delta_{\rm LAF} \sim U$, $\Delta_{\rm QAH} \sim V_2$ and $U > V_2$.
